# Supplementary material for: FairML: A Julia Package for Fair Classification
Source: arXiv:2412.01585 source file (2024-12-09)
Supplement: Supplementary file 1 [file appendix.tex]

\section{Package Documentation}
\label{sec:chapter-sensitivity}

Since the package provides the option to generate synthetic datasets for users to test any algorithms they have developed, as a in-processing phase, some auxiliary functions will help in this journey. Below is the documentation of functions that calculate and compare both fairness and regular metrics of a prediction with the original data labels.

\begin{listing}[H]
\caption{Metrics Function.}
\label{APP1}
\begin{minted}[breaklines,escapeinside=||,mathescape=true, linenos, numbersep=3pt, gobble=2, frame=lines, fontsize=\small, framesep=2mm]{julia}
function final_metrics(ynewdata::Vector{Union{Float64,
Int64}}, predictions::Vector{Union{Float64, Int64}})
    return Accuracy, FPR, FNR, TPR, TNR, Recall, TP, FP, TN, FN
end
\end{minted}
\end{listing}

\begin{listing}[H]
\caption{Fair Disparate Impact Function.}
\label{APP2}
\begin{minted}[breaklines,escapeinside=||,mathescape=true, linenos, numbersep=3pt, gobble=2, frame=lines, fontsize=\small, framesep=2mm]{julia}
function disparate_impact_metric(newdata::DataFrame, predictions::Vector{Union{Float64, Int64}}, SF::String)
    return DI_metric
end
\end{minted}
\end{listing}

\begin{listing}[H]
\caption{Fair False Negative Rate Function.}
\label{APP3}
\begin{minted}[breaklines,escapeinside=||,mathescape=true, linenos, numbersep=3pt, gobble=2, frame=lines, fontsize=\small, framesep=2mm]{julia}
function false_negative_rate_metric(newdata::DataFrame, ynewdata::Vector{Union{Float64, Int64}}, predictions::Vector{Union{Float64, Int64}}, SF::String)
    return FNR_Metric
end
\end{minted}
\end{listing}

\begin{listing}[H]
\caption{Fair False Positive Rate Function.}
\label{APP4}
\begin{minted}[breaklines,escapeinside=||,mathescape=true, linenos, numbersep=3pt, gobble=2, frame=lines, fontsize=\small, framesep=2mm]{julia}
function false_positive_rate_metric(newdata::DataFrame, ynewdata::Vector{Union{Float64, Int64}}, predictions::Vector{Union{Float64, Int64}}, SF::String)
    return FPR_Metric
end
\end{minted}
\end{listing}

\begin{listing}[H]
\caption{Fair True Negative Rate Function.}
\label{APP5}
\begin{minted}[breaklines,escapeinside=||,mathescape=true, linenos, numbersep=3pt, gobble=2, frame=lines, fontsize=\small, framesep=2mm]{julia}
function true_negative_rate_metric(newdata::DataFrame, ynewdata::Vector{Union{Float64, Int64}}, predictions::Vector{Union{Float64, Int64}}, SF::String)
    return TNR_Metric
end
\end{minted}
\end{listing}

\begin{listing}[H]
\caption{Fair True Positive Rate Function.}
\label{APP6}
\begin{minted}[breaklines,escapeinside=||,mathescape=true, linenos, numbersep=3pt, gobble=2, frame=lines, fontsize=\small, framesep=2mm]{julia}
function true_positive_rate_metric(newdata::DataFrame, ynewdata::Vector{Union{Float64, Int64}}, predictions::Vector{Union{Float64, Int64}}, SF::String)
    return TPR_Metric
end
\end{minted}
\end{listing}

\begin{listing}[H]
\caption{Fair Disparate Mistreatment Function.}
\label{APP7}
\begin{minted}[breaklines,escapeinside=||,mathescape=true, linenos, numbersep=3pt, gobble=2, frame=lines, fontsize=\small, framesep=2mm]{julia}
function disparate_mistreatment_metric(newdata::DataFrame, ynewdata::Vector{Union{Float64, Int64}}, predictions::Vector{Union{Float64, Int64}}, SF::String)
    return DM_Metric
end
\end{minted}
\end{listing}

The developed package also includes functions related to the optimization problems of regular logistic regression and support vector machines, that is, without fairness constraints, as follows:

\begin{listing}[H]
\caption{Regular Logistic Regression Function.}
\label{IDLR}
\begin{minted}[breaklines,escapeinside=||,mathescape=true, linenos, numbersep=3pt, gobble=2, frame=lines, fontsize=\small, framesep=2mm]{julia}
function di_logreg(xtrain::DataFrame, ytrain::Vector{Union{Float64, Int64}}, newdata::DataFrame, SF::Union{String, Array{String}}, c::Real)
    return prob_train, prob_newdata
end
\end{minted}
\end{listing}

\begin{listing}[H]
\caption{Regular Support Vector Machine Function.}
\label{IDSVM}
\begin{minted}[breaklines,escapeinside=||,mathescape=true, linenos, numbersep=3pt, gobble=2, frame=lines, fontsize=\small, framesep=2mm]{julia}
function di_logreg(xtrain::DataFrame, ytrain::Vector{Union{Float64, Int64}}, newdata::DataFrame, SF::Union{String, Array{String}}, c::Real)
    return prob_train, prob_newdata
end
\end{minted}
\end{listing}

\begin{listing}[H]
\caption{Mixed Effects Support Vector Machine Function.}
\label{IDMELR}
\begin{minted}[breaklines,escapeinside=||,mathescape=true, linenos, numbersep=3pt, gobble=2, frame=lines, fontsize=\small, framesep=2mm]{julia}
function id_me_logreg(xtrain::DataFrame, ytrain::Vector{Union{Float64, Int64}}, newdata::DataFrame, SF::Union{String, Array{String}}, c::Real, group_id_train::CategoricalVector, group_id_newdata::CategoricalVector)
    return prob_train, prob_newdata
end
\end{minted}
\end{listing}

\begin{listing}[H]
\caption{Mixed Effects Support Vector Machine Function.}
\label{IDMESVM}
\begin{minted}[breaklines,escapeinside=||,mathescape=true, linenos, numbersep=3pt, gobble=2, frame=lines, fontsize=\small, framesep=2mm]{julia}
function id_me_svm(xtrain::DataFrame, ytrain::Vector{Union{Float64, Int64}}, newdata::DataFrame, SF::Union{String, Array{String}}, c::Real, group_id_train::CategoricalVector, group_id_newdata::CategoricalVector)
    return prob_train, prob_newdata
end
\end{minted}
\end{listing}
